# Supplementary material for: Weaves, Wires, and Morphisms: Formalizing and Implementing the Algebra of Deep Learning
Source: arXiv:2604.07242 source file (2026-08-12)
Supplement: Supplementary file 1 [file 2Category_Appendix.tex]

\documentclass[../main-source.tex]{subfiles}
\graphicspath{{\subfix{../figures/}}}

\begin{document}
\subsection{Remapping Algebra}

Parallelism with respect to discrete functions is offered by the \textbf{direct sum}, which concatenates maps $\displaystyle \mu :J\rightarrow I$ and $\displaystyle \nu :K\rightarrow L$ into a map $\displaystyle \mu \oplus \nu :J\oplus K\rightarrow L\oplus I$. This satisfies the conditions of a monoidal product, though our lone objects approach would require objects $\displaystyle n$ to be expressed as $\displaystyle \oplus _{i\in n}\mathbf{1}$ to not have redundancy in objects. If we express discrete functions as tuples $\displaystyle \mu \sim I^{J}$, then the discrete sum is given by tuple concatenation. Direct sums of remappings gives the product of rearrangements. This can be provided by Definition~\ref{def:product_category}, or follow from the elemental category element properties of Definition~\ref{def:elemental}. The direct sum of discrete functions is shown in Definition~\ref{def:dsum}, diagrammed in Figure~\ref{fig:appendix0_dsum}, along with correspondence to rearrangements.

\begin{definition}

[Direct Sum of Discrete Functions]\label{def:dsum}
Given a family of discrete functions $\displaystyle ( \mu _{i})_{i\in I}$ where $\displaystyle \mu _{i} :P_{i}\rightarrow Q_{i}$, the \textbf{direct sum};

\begin{equation}
\displaystyle ( \oplus _{i\in I} \mu _{i}) :\Sigma _{i\in I} P_{i}\rightarrow \Sigma _{i\in I} Q_{i} \label{eq:dsum}
\end{equation}

Is defined so that for $\displaystyle s\in I$ (segment choice) and $\displaystyle \ell \in P_{s}$ (offset) we have;

\begin{equation}
( \oplus _{i\in I} \mu _{i})( \ell +\Sigma _{i\in s} P_{i}) =\mu _{s}( \ell ) +\Sigma _{i\in s} Q_{i}
\label{eq:dsum_expr}
\end{equation}

\end{definition}

\DiagramMacroCtwo{2Category}{appendix0_dsum}{
The direct sum of discrete functions concatenates their mappings, and is given by offsetting latter functions. This corresponds to the product of rearrangements.
}{appendix0_dsum_rearrangements}

Naturality applies to products of morphisms in general. For $f_i:A_i\to B_i$ where naturality provides $(\Pi_{i\in I} f_i) \compose [\mu]_{(B_i)_{i\in I}} = [\mu]_{(A_i)_{i \in I}}\compose (\Pi_{j \in J} f_{\mu(j)})$ applies just as well to $B_i$ being singular or product objects. Therefore, we need a mechanism for expressing this form of naturality, and we provide this by offsets provided in Definition~\ref{def:flatten}.

\begin{definition}
[Associativity Compatibility]\label{def:flatten}
A remapping can be made \textit{flat}. If we have a remapping $\displaystyle \mu :J\rightarrow I$ and target sizes $\displaystyle ( L_{i})_{i\in I}$, then we define;

\begin{equation}
 \displaystyle \mu _{( L_{i})_{i\in I}} :\Sigma _{j\in J} L_{\mu ( j)}\rightarrow \Sigma _{i\in I} L_{i} \label{eq:flatten}
\end{equation}

So that for $\displaystyle s\in J$ (segment choice) and $\displaystyle \ell \in L_{\mu ( s)}$ (offset) we have (using bra-notation $\displaystyle \bra{\square}$ to indicate elements clearly);

\begin{equation}
\bra{\ell +\Sigma _{j\in s} L_{\mu ( j)}} \compose \mu _{( L_{i})_{i\in I}} =\bra{\ell +\Sigma _{i\in \mu ( s)} L_{i}}
\label{eq:flatten_expr}
\end{equation}

A remapping $\displaystyle \mu :J\rightarrow I$ over a family of flat objects $\displaystyle ( A_{i})_{i\in I}$ so that $\displaystyle A_{i} =\Pi _{k\in L_{i}} A_{ik}$ is defined so that;

\begin{align*}
[ \mu ]_{( \Pi _{k\in L[ A_{i}]} A_{ik})_{i\in I}} & =[ \mu _{( L[ A_{i}])_{i\in I}}]_{( A_{ik})_{i\in I,k\in L[ A_{i}]}}
\end{align*}

Naturality for an $\displaystyle I$-family of morphisms $\displaystyle ( f_{i})_{i\in I}$ where $\displaystyle f_{i} :A_{i}\rightarrow B_{i}$ ($\displaystyle A_{i}$ and $\displaystyle B_{i}$ are flat objects with some length) can then be more precisely expressed as;

\begin{align*}
( \Pi _{i\in I} f_{i}) \compose [ \mu ]_{( B_{i})_{i\in I}} 
& =[ \mu ]_{( A_{i})_{i\in I}} \compose ( \Pi _{j\in J} f_{\mu ( j)})
\\
( \Pi _{i\in I} f_{i}) \compose [ \mu _{( L[ B_{i}])_{i\in I}}]_{( B_{ik})_{i\in I,k\in L_{i}}} 
& =[ \mu _{( L[ A_{i}])_{i\in I}}]_{( A_{ik})_{i\in I,k\in L_{i}}} \compose ( \Pi _{j\in J} f_{\mu ( j)})
\end{align*}

In implementations, we will be working with flat remappings.

\end{definition}

\end{document}
