# Supplementary material for: Weaves, Wires, and Morphisms: Formalizing and Implementing the Algebra of Deep Learning
Source: arXiv:2604.07242 source file (2026-08-12)
Supplement: Supplementary file 2 [file Appendix_Fox.tex]

\documentclass[../main-source.tex]{subfiles}
\graphicspath{{\subfix{../figures/}}}

\begin{document}
\subsection{Fox's Theorem}

Fox's theorem relates the naturality of a product category to the algebraic properties and degrees of freedom of its morphisms. The classical result from~\cite{fox1976coalgebras} relates Cartesian to monoidal categories. We split the result into two sections, relating it to the properties of copying (unique identification) and deletion (free construction).

\begin{theorem} \label{thm:fox}
[Fox's Theorem] We split Fox's theorem into two parts, relating naturality properties to aspects of Cartesian products. For a copy-discard category where all rearrangements are allowed we have;

\begin{itemize}
\item \textbf{Unique Identification} If copying (count increases) are natural, then for morphisms $\displaystyle f:A\rightarrow \Pi _{i\in I} B_{i}$ and $\displaystyle g:A\rightarrow \Pi _{i\in I} B_{i}$ if for all remappings $\displaystyle i:\mathbf{1}\rightarrow i$ we have $\displaystyle f\compose [ i] =g\compose [ i]$, then $\displaystyle f=g$. This supplies an injective map $\displaystyle \mathcal{C}( A,\Pi _{i\in I} B_{i})\rightarrow \Pi _{i\in I}\mathcal{C}( A,B_{i})$.
\item \textbf{Free Construction }If deletion (count decreases) are natural, then for an $\displaystyle I$-family of morphisms $\displaystyle ( f_{i})_{i\in I}$ where $\displaystyle f_{i} :A\rightarrow B_{i}$, there exists a morphism $\displaystyle F:A\rightarrow \Pi _{i\in I} B_{i}$ so that for remappings $\displaystyle i:\mathbf{1}\rightarrow i$ we have $\displaystyle F\compose [ i] =f_{i}$. This supplies an injective map $\displaystyle \Pi _{i\in I}\mathcal{C}( A,B_{i})\rightarrow \mathcal{C}( A,\Pi _{i\in I} B_{i})$.
\end{itemize}

Together, these properties describe a Cartesian product and indicate a bijective map $\displaystyle \mathcal{C}( A,\Pi _{i\in I} B_{i}) \sim \Pi _{i\in I}\mathcal{C}( A,B_{i})$.

\end{theorem}

For the proof, the high-level idea is to first construct an identity using a copy followed by selective projections, given by;

\begin{align}
[ \delta ^{I}]_{( \Pi _{i\in I} B_{i})_{b\in \mathbf{1}}} \compose \Pi _{a\in I}[ a]_{( B_{i})_{i\in I}} & =\text{Id}[ \Pi _{i\in I} B_{i}] \label{eq:idrearrangement}
\end{align}

The case of $I=\mathbf{2}$ can be diagrammed by;
\begin{center}
\tablefig{Appendix/appendix_idrearrangement}
\end{center}

As a morphism followed by an identity is itself, applying this construct provides a bijective map on morphisms.

\begin{proof}

We will show that;

\begin{align*}
[ \delta ^{I}]_{( \Pi _{i\in I} B_{i})_{b\in \mathbf{1}}} \compose \prod _{a\in I}[ a]_{( B_{i})_{i\in I}} & =\text{Id}[ \Pi _{i\in I} B_{i}]
\end{align*}

We have our rearrangements supplied by;

\begin{align*}
\delta ^{I} & :I\rightarrow \mathbf{1} & [ \delta ^{I}]_{\Pi _{i\in I} B_{i}} & :\Pi _{i\in I} B_{i}\rightarrow \Pi _{a\in I} \Pi _{i\in I} B_{i}\\
\bra{a} & :\mathbf{1}\rightarrow I & [ a]_{( B_{i})_{i\in I}} & :\Pi _{i\in I} B_{i}\rightarrow B_{a}\\
 &  & \prod _{a\in I}[ a]_{( B_{i})_{i\in I}} & :\Pi _{a\in I} \Pi _{i\in I} B_{i}\rightarrow \Pi _{a\in I} B_{a}
\end{align*}

The product and composition exclusively of rearrangements is defined by their underlying remapping, and therefore is the same in all product categories where the rearrangements are allowed. This allows us to use product naturality rules. Acting on this expression with an element $\displaystyle \bra{c} :\mathbf{1}\rightarrow I$ as a projection $\displaystyle [ c]_{( B_{a})_{a\in I}} :\Pi _{a\in I} B_{a}\rightarrow B_{c}$ we get;

\begin{align*}
[ \delta ^{I}]_{\Pi _{i\in I} B_{i}} \compose \underbrace{\left(\prod _{a\in I}[ a]_{( B_{i})_{i\in I}}\right) \compose [ c]_{( B_{a})_{a\in I}}}_{\text{Extract } a=c} & =\underbrace{[ \delta ^{I}]_{\Pi _{i\in I} B_{i}} \compose [ c]_{( \Pi _{i\in I} B_{i})_{a\in I}}}_{\text{Compatible}} \compose [ c]_{( B_{i})_{i\in I}}\\
 & =[ c\compose \delta ^{I}]_{\Pi _{i\in I} B_{i}} \compose [ c]_{( B_{i})_{i\in I}}\\
 & =[\text{Id}_{\mathbf{1}}]_{\Pi _{i\in I} B_{i}} \compose [ c]_{( B_{i})_{i\in I}}\\
 & =[ c]_{( B_{i})_{i\in I}}
\end{align*}

Therefore, the rearrangement $\displaystyle [ \delta ^{I}]_{( \Pi _{i\in I} B_{i})_{b\in \mathbf{1}}} \compose \Pi _{a\in I}[ a]_{( B_{i})_{i\in I}}$ has a remapping which maps each $\displaystyle \bra{c} :\mathbf{1}\rightarrow I$ to $\displaystyle \bra{c} :\mathbf{1}\rightarrow I$, and is therefore the identity.

\end{proof}

We can now prove unique identification. We will correspond equations with diagrams for the case of $I=2$.

\begin{proof}

We take two morphisms $\displaystyle f,g:A\rightarrow \Pi _{i\in I} B_{i}$ where for all elements $\displaystyle \bra{a} :\mathbf{1}\rightarrow I$ we have $\displaystyle f\compose [ a]_{( B_{i})_{i\in I}} =g\compose [ a]_{( B_{i})_{i\in I}}$. Therefore, we have;

\begin{align*}
\left(\prod _{a\in I} f\compose [ a]_{( B_{i})_{i\in I}}\right) & =\left(\prod _{a\in I} g\compose [ a]_{( B_{i})_{i\in I}}\right)\\
[ \delta ^{I}]_{A} \compose \prod _{a\in I} f\compose \prod _{a\in I}[ a]_{( B_{i})_{i\in I}} & =[ \delta ^{I}]_{A} \compose \prod _{a\in I} g\compose \prod _{a\in I}[ a]_{( B_{i})_{i\in I}}
\end{align*}

This corresponds to the diagrams;

\begin{center}
\tablefig{Appendix/appendix_uid0}
\tablefig{Appendix/appendix_uid1}
\end{center}

If count increases are natural, then we apply;

\begin{align*}
f\compose [ \delta ^{I}]_{\Pi _{i\in I} B_{i}} \compose \prod _{a\in I}[ a]_{( B_{i})_{i\in I}} & =g\compose [ \delta ^{I}]_{\Pi _{i\in I} B_{i}} \compose \prod _{a\in I}[ a]_{( B_{i})_{i\in I}}\\
f\compose \text{Id}[ \Pi _{i\in I} B_{i}] & =g\compose \text{Id}[ \Pi _{i\in I} B_{i}] \ \left(\text{Eq. }\ref{eq:idrearrangement}\right)\\
f & =g
\end{align*}

Corresponding to the diagrams;
\begin{center}
\tablefig{Appendix/appendix_uid2}
\tablefig{Appendix/appendix_uid3}
\end{center}

Therefore, if for all elements $\displaystyle \bra{a} :\mathbf{1}\rightarrow I$ we have $\displaystyle f\compose [ a]_{( B_{i})_{i\in I}} =g\compose [ a]_{( B_{i})_{i\in I}}$, in a natural copying category, then $\displaystyle f=g$. This provides an injective map from $\displaystyle \mathcal{C}( A,\Pi _{i\in I} B_{i})$ to a family of morphisms $\displaystyle \Pi _{i\in I}\mathcal{C}( A,B_{i})$.

\end{proof}

Finally, we derive free construction from natural deletion / count decreases.

\begin{proof}

Given a family of morphisms $\displaystyle ( f_{i})_{i\in I}$ where $\displaystyle f_{i} :A\rightarrow B_{i}$, we define;

\begin{align*}
F & =[ \delta ^{I}]_{A} \compose \left(\prod _{a\in I} f_{a}\right)
\end{align*}

If count decreases (deletion) is natural, then we can apply a rearrangement generated by an element $\displaystyle \bra{c} :\mathbf{1}\rightarrow I$ to get;

\begin{align*}
F\compose [ c]_{( B_{a})_{a\in I}} & =[ \delta ^{I}]_{A} \compose \left(\prod _{a\in I} f_{a}\right) \compose [ c]_{( B_{a})_{a\in I}}\\
 & =[ \delta ^{I}]_{A} \compose [ c]_{( A)_{a\in I}} \compose f_{c}\\
 & =[\text{Id}_{\mathbf{1}}]_{A} \compose f_{c}\\
 & =f_{c}
\end{align*}

Therefore, we can construct a morphism $\displaystyle F:A\rightarrow \Pi _{i\in I} B_{i}$ so that $\displaystyle F\compose [ c]_{( B_{a})_{a\in I}} =f_{c}$ for all $\displaystyle \bra{c} :\mathbf{1}\rightarrow I$. This provides an injective map from families of morphisms $\Pi_{i \in I} \mathcal{C}(A,B_i)$ to $\mathcal{C}(A,\Pi_{i\in I}B_i)$.

\end{proof}

\end{document}
