# Supplementary material for: Weaves, Wires, and Morphisms: Formalizing and Implementing the Algebra of Deep Learning
Source: arXiv:2604.07242 source file (2026-08-12)
Supplement: Supplementary file 3 [file Appendix_Results.tex]

\documentclass[../main-source.tex]{subfiles}
\graphicspath{{\subfix{../figures/}}}

\begin{document}

\section{Results Notebook}\label{sec:jupyter}
\begin{figure}[h]
    \centering
    \begin{minipage}{0.5\textwidth}
        \centering
        \includegraphics[width=\textwidth]{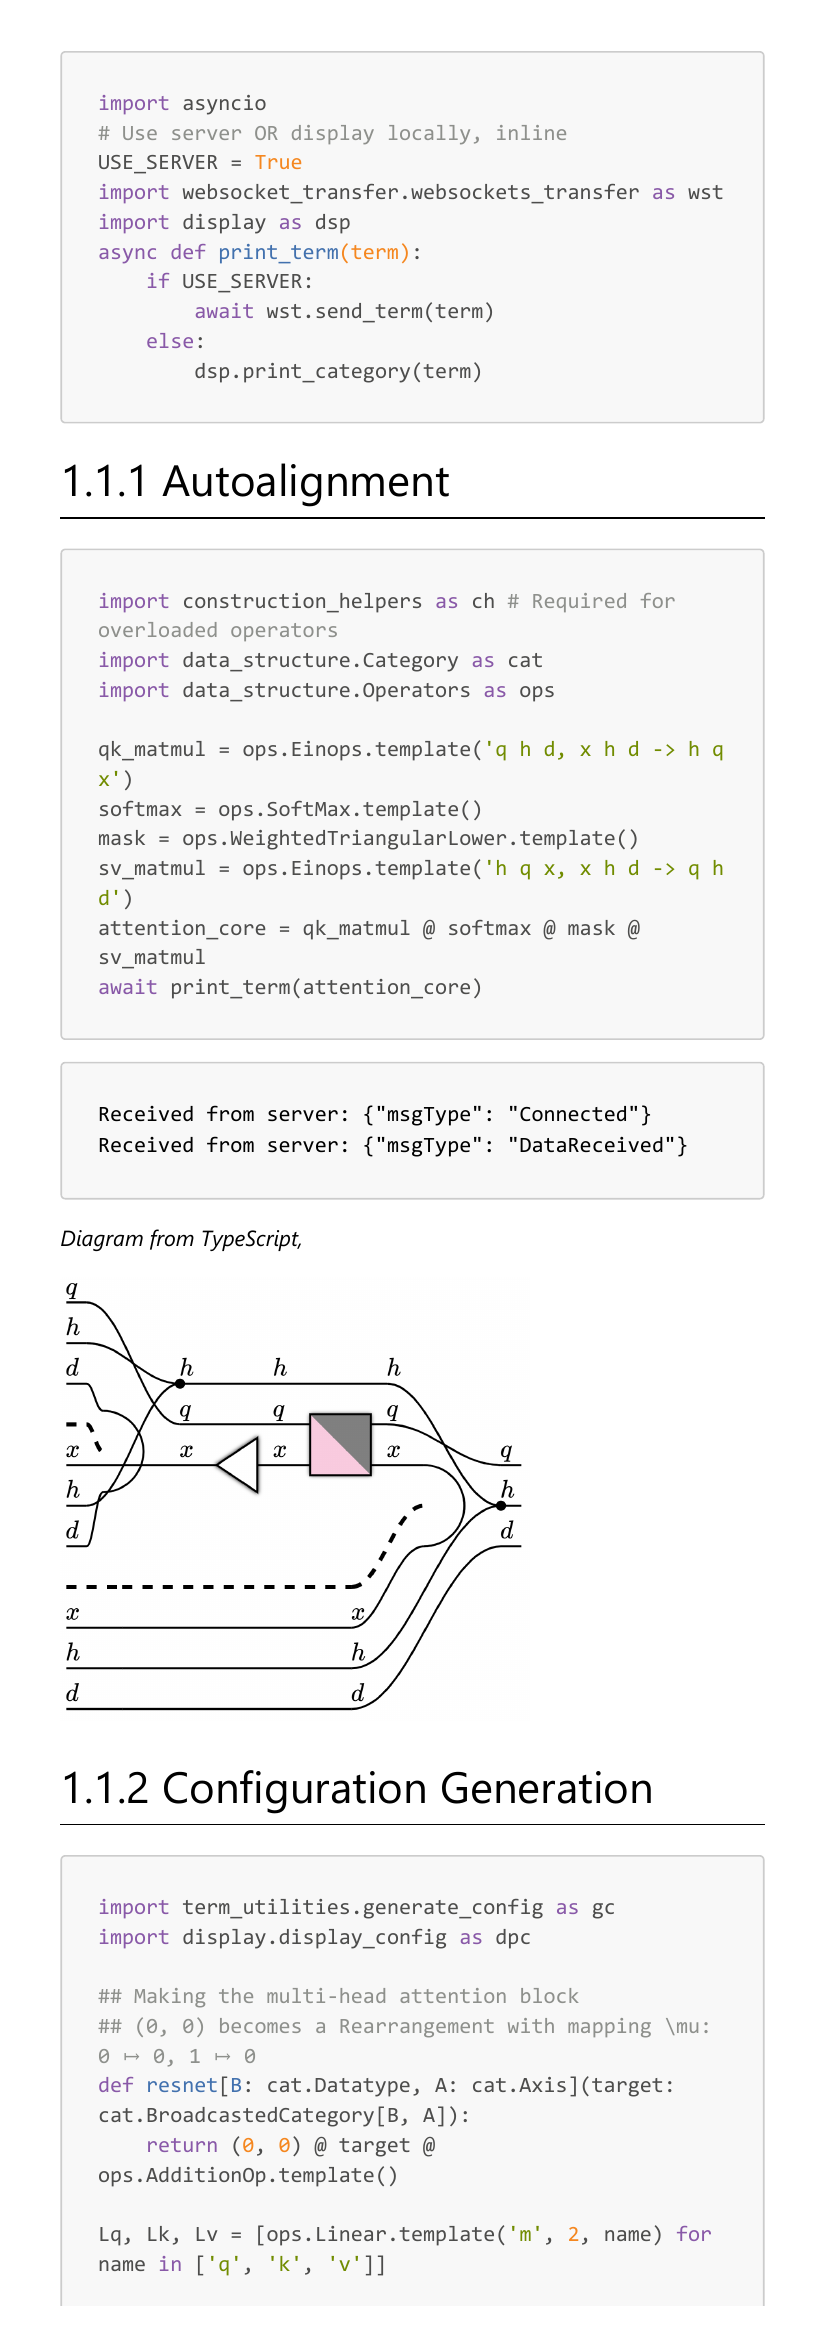} %
    \end{minipage}%
    \begin{minipage}{0.5\textwidth}
        \centering
        \includegraphics[width=\textwidth]{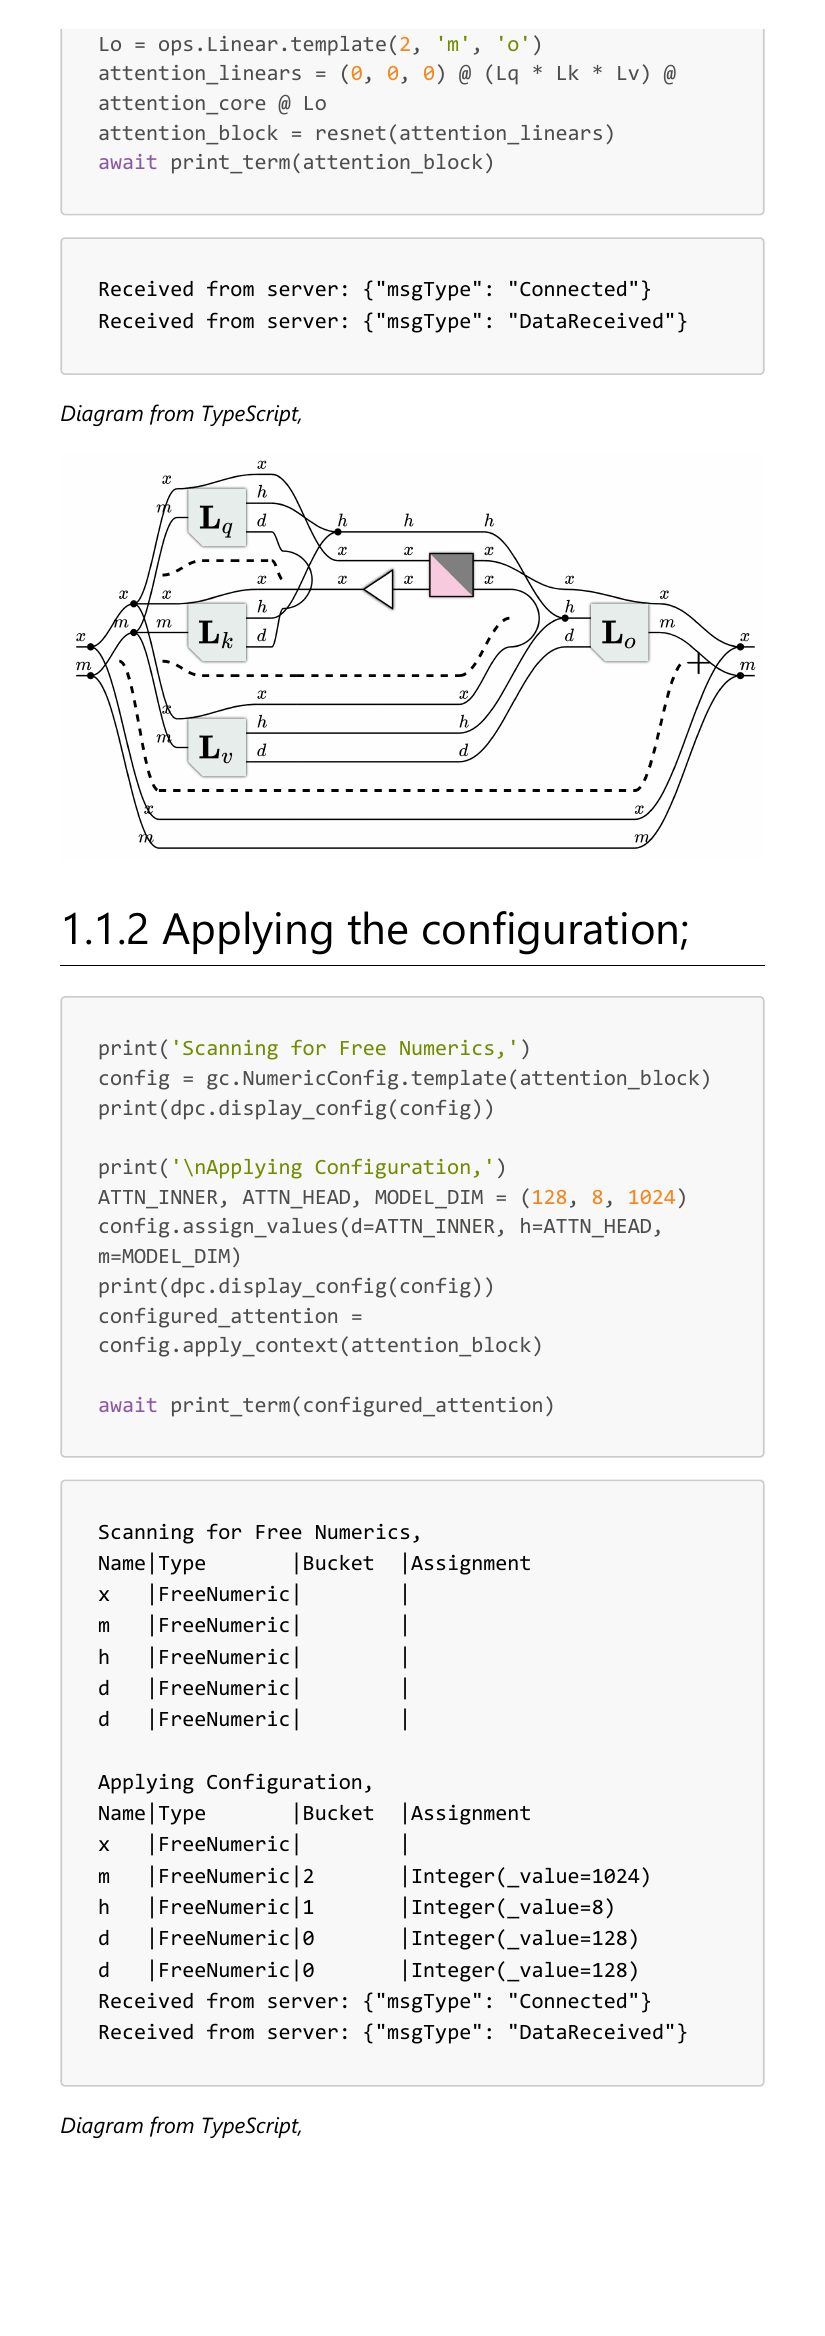} %
    \end{minipage}
\end{figure}
\begin{figure}[h]
    \centering
    \begin{minipage}{0.5\textwidth}
        \centering
        \includegraphics[width=\textwidth]{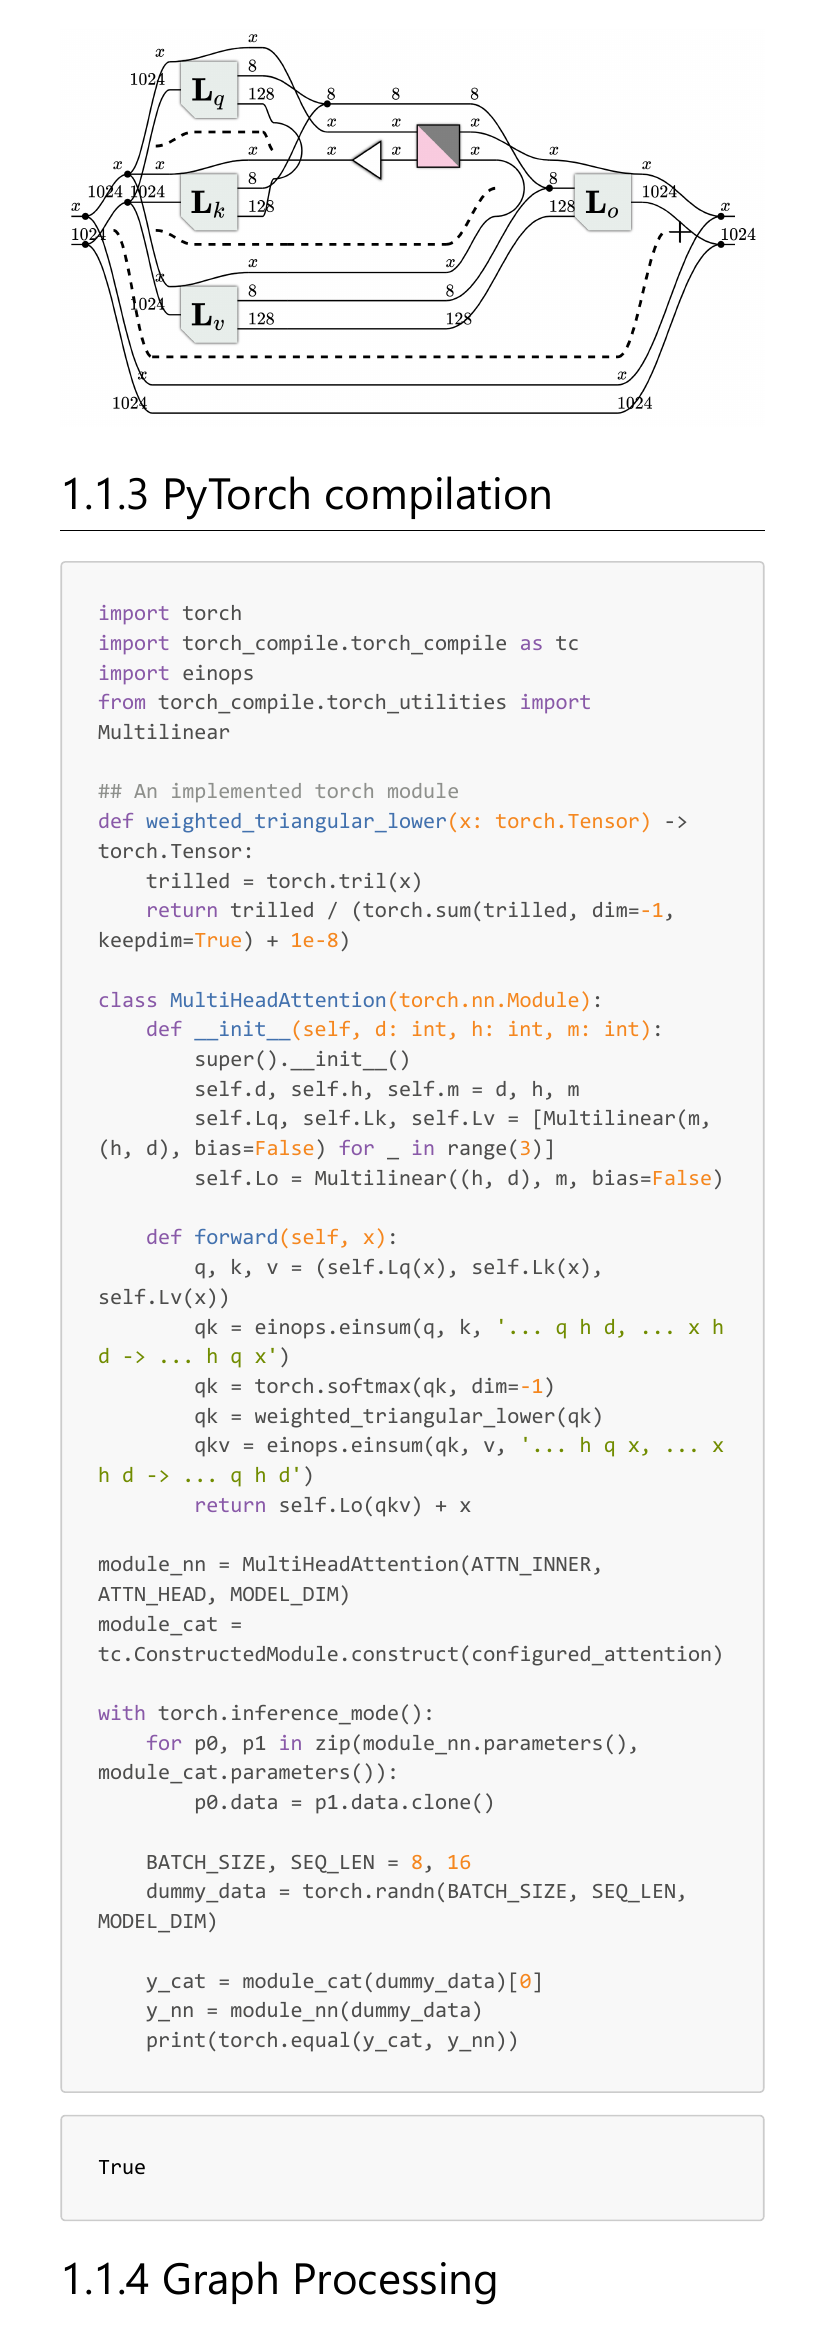} %
    \end{minipage}%
    \begin{minipage}{0.5\textwidth}
        \centering
        \includegraphics[width=\textwidth]{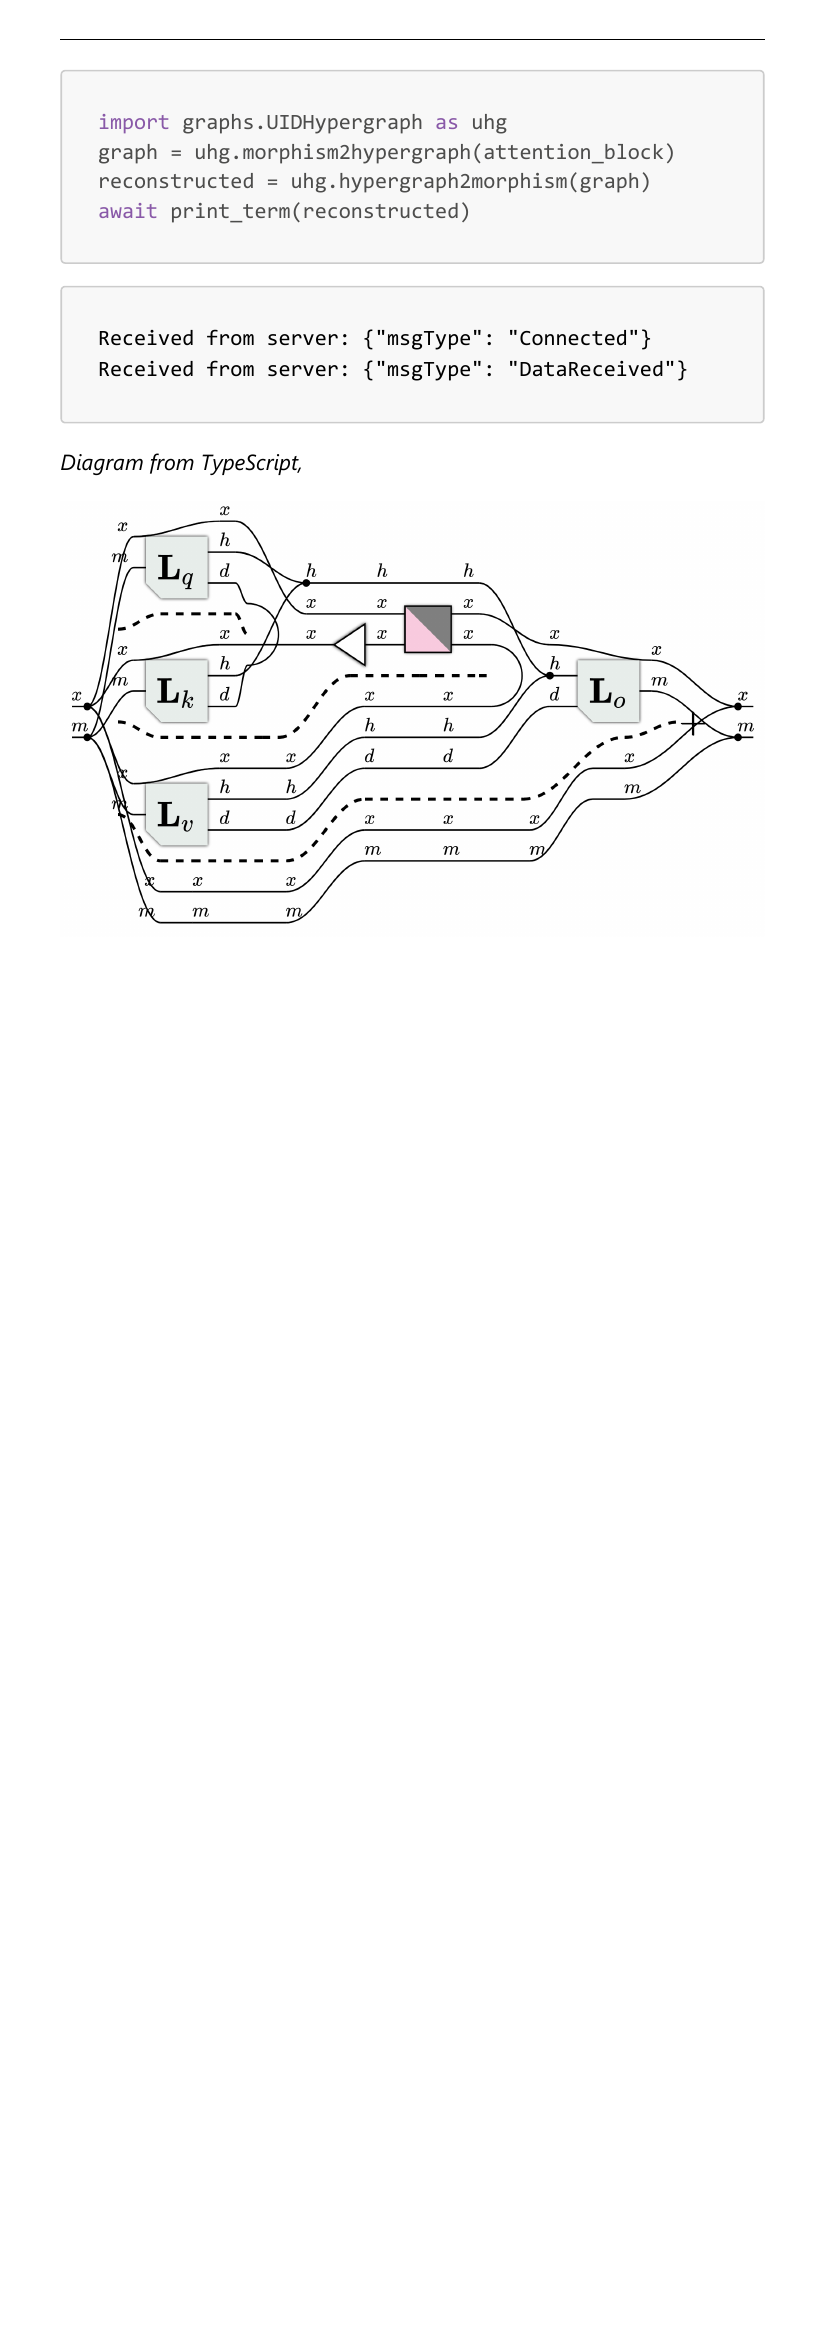} %
    \end{minipage}
\end{figure}

\end{document}
