# Supplementary material for: Weaves, Wires, and Morphisms: Formalizing and Implementing the Algebra of Deep Learning
Source: arXiv:2604.07242 source file (2026-08-12)
Supplement: Supplementary file 4 [file Appendix_Yoneda.tex]

\documentclass[../main-source.tex]{subfiles}
\graphicspath{{\subfix{../figures/}}}

\begin{document}
\subsection{Deterministic Naturality}
In an elemental category, deterministic morphisms which map elements to elements are universally natural, owing to the naturality of elements. Rearrangements on elements $\displaystyle ( a_{i})_{i\in I}$ so that $\displaystyle a_{i} \in \text{El}( A_{i})$ are defined so that;

\begin{align*}
\left(\prod _{i\in I} a_{i}\right) \compose [ \mu ]_{( A_{i})_{i\in I}} & =\left(\prod _{j\in J} a_{\mu ( j)}\right)
\end{align*}

Consider a family of deterministic morphisms $\displaystyle ( f_{i})_{i\in I}$ so that $\displaystyle f_{i} :A_{i}\rightarrow B_{i}$. Determinism (see Definition~\ref{def:elemental}) maps elements to elements, so for an element $\displaystyle a_{i} \in \text{El}( A_{i})$ we have $\displaystyle a_{i} \compose f_{i} \in \text{El}( B_{i})$. Therefore, we have;
\begin{align}
\left(\prod _{i\in I} f_{i}\right) \compose [ \mu ]_{( B_{i})_{i\in I}} & =[ \mu ]_{( A_{i})_{i\in I}} \compose \left(\prod _{j\in J} f_{\mu ( j)}\right) \label{eq:detnat}
\end{align}
As we have for the left-hand side;
\begin{align*}
\left(\prod _{i\in I} a_{i}\right) \compose ( LHS) & =\left(\prod _{i\in I} a_{i}\right) \compose \left(\prod _{i\in I} f_{i}\right) \compose [ \mu ]_{( B_{i})_{i\in I}}\\
 & =\left(\prod _{i\in I}( a_{i} \compose f_{i})\right) \compose [ \mu ]_{( B_{i})_{i\in I}}\\
 & =\left(\prod _{j\in J}( a_{\mu ( j)} \compose f_{\mu ( j)})\right)
\end{align*}
And the right-hand side;
\begin{align*}
\left(\prod _{i\in I} a_{i}\right) \compose ( RHS) & =\left(\prod _{i\in I} a_{i}\right) \compose [ \mu ]_{( A_{i})_{i\in I}} \compose \left(\prod _{j\in J} f_{\mu ( j)}\right)\\
 & =\left(\prod _{j\in J} a_{\mu ( j)}\right) \compose \left(\prod _{j\in J} f_{\mu ( j)}\right) =\left(\prod _{j\in J} a_{\mu ( j)} \compose f_{\mu ( j)}\right)
\end{align*}
Therefore, the left- and right-hand sides are equal as they have the same action on elements, and deterministic morphisms are natural over all rearrangements.

\subsection{Yoneda Sliding}~\label{sec:yoneda}
The Yoneda lemma describes how we can naturally transform between functors, composition preserving maps between morphisms. In our case, it corresponds to reindexing slides as seen in Figure~\ref{fig:addops11_convolution_equivariance}. As we are not strictly enforcing the Cartesian property, we are working outside $\displaystyle \mathbf{Set}$ and therefore the Yoneda lemma only applies under certain cases.

\begin{theorem}[Yoneda Sliding]
In the array-broadcasted category $\displaystyle \mathbf{Br}$, given a morphism $\displaystyle f:X\rightarrow Y\in \text{Mo}\mathbf{Br}$ and a stride morphism $\displaystyle \eta :P\rightarrow Q\in \text{Mo}\mathbf{St}$, where either (a) the morphism is deterministic, or (b) the stride morphism provides a natural remapping, we have Yoneda sliding given by;
\begin{align}
[ X,\eta ] \compose [ f,P] & =[ f,Q] \compose [ Y,\eta ] \label{eq:yoneda}
\end{align}
This can be diagrammed by;
\begin{center}
\tablefig{Appendix/appendix0_yoneda}
\end{center}

\end{theorem}

\begin{proof}
We consider the extracted case, applying $\displaystyle [ \delta ^{P}]_{[ Y,P]} \compose \Pi _{p\in \text{El}( P)}[ Y,p]$ to both sides. This gives us;
\begin{align*}
( LHS) & =[ X,\eta ] \compose [ f,P] \compose [ \delta ^{P}]_{[ Y,P]} \compose \left(\prod _{p\in \text{El}( P)}[ Y,p]\right)\\
 & =[ X,\eta ] \compose [ \delta ^{P}]_{[ X,P]} \compose \left(\prod _{p\in \text{El}( P)}[ X,p] \compose f\right) \ \left(\text{Eq. } \ref{eq:batchparallel}\right)\\
 & =[ \delta ^{P}]_{[ X,Q]} \compose \left(\prod _{p\in \text{El}( P)}[ X,\eta ] \compose [ X,p] \compose f\right) \ \left(\text{Eq. } \ref{eq:detnat}\right)\\
 & =[ \delta ^{P}]_{[ X,Q]} \compose \left(\prod _{p\in \text{El}( P)}[ X,\eta ( p)] \compose f\right) \ \left(\text{Eq. } \ref{eq:reindexing} \right)
\end{align*}
For the right-hand-side, we use the fact that;
\begin{equation}
[ \delta ^{P}]_{[ Y,P]} \compose \left(\prod _{p\in \text{El}( P)}[ Y,\eta ( p)]\right) =[ \delta ^{Q}]_{[ Y,P]} \compose \left(\prod _{q\in \text{El}( Q)}[ Y,q]\right) \compose [ \eta ]_{( Y)_{q\in Q}} \label{eq:indexrearrangement}
\end{equation}
Which we can show by taking an element $\displaystyle y\in \text{El}[ Y,P]$,
\begin{align*}
y\compose [ \delta ^{P}]_{[ Y,P]} \compose \left(\prod _{p\in \text{El}( P)}[ Y,\eta ( p)]\right) & =\left(\prod _{p\in \text{El}( P)} y\compose [ Y,\eta ( p)]\right)\\
y\compose [ \delta ^{Q}]_{[ Y,P]} \compose \left(\prod _{q\in \text{El}( Q)}[ Y,q]\right) \compose [ \eta ]_{( Y)_{q\in Q}} & =\left(\prod _{q\in \text{El}( Q)} y\compose [ Y,q]\right) \compose [ \eta ]_{( Y)_{q\in Q}}\\
 & =\left(\prod _{p\in \text{El}( P)} y\compose [ Y,\eta ( p)]\right)
\end{align*}
Therefore, we have;
\begin{align*}
( RHS) & =[ f,Q] \compose [ Y,\eta ] \compose [ \delta ^{P}]_{[ Y,P]} \compose \left(\prod _{p\in \text{El}( P)}[ Y,p]\right)\\
 & =[ f,Q] \compose [ \delta ^{P}]_{[ Y,P]} \compose \left(\prod _{p\in \text{El}( P)}[ Y,\eta ( p)]\right) \ \left(\text{Eq. } \ref{eq:detnat}, \ref{eq:reindexing}\right)\\
 & =[ f,Q] \compose [ \delta ^{Q}]_{[ Y,P]} \compose \left(\prod _{q\in \text{El}( Q)}[ Y,q]\right) \compose [ \eta ]_{( Y)_{q\in Q}} \ \left(\text{Eq. } \ref{eq:indexrearrangement} \right)\\
 & =[ \delta ^{Q}]_{[ X,P]} \compose \left(\prod _{q\in \text{El}( Q)}[ X,q] \compose f\right) \compose [ \eta ]_{( Y)_{q\in Q}}
\end{align*}
This shows how the two expressions differ. Using $\displaystyle [ f,P]$ as opposed to $\displaystyle [ f,Q]$ determines how many times the underlying operation is run in parallel. This has implications for the degrees of independence of the output, computational cost, or other ``non-functional'' factors which are overlooked in an all-natural $\displaystyle \mathbf{Set}$ based approach.

If we now assume that either $\displaystyle f$ is deterministic, and therefore is natural with respect to all remappings, or that $\displaystyle \eta :P\rightarrow Q$ provides a natural remapping, then the $\displaystyle RHS$ further simplifies;
\begin{align*}
( RHS) & =[ \delta ^{Q}]_{[ X,P]} \compose [ \eta ]_{( Y)_{q\in Q}} \compose \left(\prod _{p\in \text{El}( P)}[ X,\eta ( p)] \compose f\right)\\
 & =[ \delta ^{P}]_{[ X,P]} \compose \left(\prod _{p\in \text{El}( P)}[ X,\eta ( p)] \compose f\right)\\
 & =( LHS)
\end{align*}
This provides index sliding. As the two sides are equal over an injective composition, we derive Equation~\ref{eq:yoneda}.
\end{proof}

\end{document}
